# Supplementary material for: Fast Verification of Strong Database Isolation (Extended Version)
Source: arXiv:2511.14067 source file (2025-11-18)
Supplement: Supplementary file 1 [file app-complexity.tex]

% complexity.tex

\section{\brown{Complexity Analysis}}
\label{section:appendix-complexity}

\zhiheng{Reviewer \#3 requires that 
a comprehensive complexity analysis 
should be included in the main text.}

\zhiheng{TODO: remove this section}

We provide a complexity analysis of \ourtool in four main stages,
following our pseudo algorithm 
(with some details in the Appendix~\cite{tech-rpt}).

\inlsec{Constructing} 
Let $\totalsize{\wwcons}$ and $\totalsize{\wrcons}$ denote the total number of 
possible $\WW$ and $\WR$ edges in $\wwcons$ and $\wrcons$, 
respectively, 
defined by  
$\totalsize{\brown{\mathcal{X}}} = \sum\limits_{\ccons \in \brown{\mathcal{X}}} \cardinality{\ccons}$ 
for $\brown{\mathcal{X}} \in \set{\wwcons, \wrcons}$.
\zhiheng{cannot use $\C$ here, which notation?}
The time complexity of constructing the hyper-polygraph is therefore 
$O(\totalsize{\wwcons} + \totalsize{\wrcons})$.

\inlsec{Pruning} 
Our pruning algorithm proceeds in iterative passes.
In each pass, it first computes reachability, 
and then enumerates constraints in $\C$ to test 
the three pruning cases illustrated in Figure~\ref{fig:pruning-cases}.
This process repeats until the known graph stabilizes.

The time complexity of computing reachability is 
$O\big(\tfrac{\cardinality{\V} \cdot \cardinality{\E}}{w}\big)$ 
where $(\V, \E)$ is the known graph and 
$w$ is the bit width used in the computation (typically $32$).
Since reachability information is cached, 
testing each pruning case costs $O(1)$, 
and the main bottleneck lies in enumerating possible $\RW$ edges.
Its complexity can be characterized by the number of four-elementary tuple 
$(T, T', S, x)$ such that 
$T, T', S \in \T, x \in \Key, T, T' \vdash \writeevent(x, \_)$ 
and $S \vdash \readevent(x, \_)$. 
We denote $\set{T \mid T \vdash \readevent(x, \_)}$ 
as $\ReadTx_x$ (symmetrically to $\WriteTx_x$).
Hence, the time complexity of each pruning pass is 
$O(\sum\limits_{x \in \Key} \cardinality{\WriteTx_x}^2 \cdot \cardinality{\ReadTx_x})$. 
Let $N_{\P}$ be the number of pruning passes.
The overall time complexity of pruning is therefore 
$O\bigl(N_{\P} \cdot \big(\tfrac{\cardinality{\V} \cdot \cardinality{\E}}{w} + 
\sum\limits_{x \in \Key} \cardinality{\WriteTx_x}^2 \cdot \cardinality{\ReadTx_x}\big)\bigr)$.

% In the worst cases, 
% the overhead of pruning is significantly high. 
% However, we \brown{argue} 
% \zhiheng{``argue'' may be too sharp} 
% that these extreme situations 
% are rare in practice. 
% In our experiments, we find that $N_{\P}$ is relatively small 
% (usually less than $10$), 
% the bitwise operations reduce the time of computing reachability to $\frac{1}{w}$, 
% and the . 

In theory, 
the overhead of pruning can be considerably large 
in the worst cases,  
primarily due to a large $N_{\P}$.
An natural upper bound for $N_{\P}$ is 
$\totalsize{\wwcons} + \totalsize{\wrcons}$ 
(i.e., only a single possible edge is eliminated in each pass).
Unfortunately, this upper bound  
can, in fact, be attained under carefully constructed scenarios.
However, we contend that 
such extreme cases are rare in practical workloads.
In our experiments, we observe that $N_{\P}$ remains relatively small 
(typically less than $10$).
Therefore, the overhead of pruning does not pose a practical concern.

\inlsec{Encoding} 
Let $\G_p = (\V_p, \E_p, (\wwcons_p, \wrcons_p))$ 
denote the hyper-polygraph after pruning. 
The encoded formula consists of two parts: 
constraints in $\C$ and clauses of 2-width cycles.
The time complexity of encoding $\C$ is 
$O(\totalsize{\wwcons_p} + \totalsize{\wrcons_p})$, 
while the time complexity of encoding 2-width cycles is 
$O(\totalsize{\wwcons_p} + \totalsize{\wrcons_p})^2)$ 
(assuming that reachability has been computed in advance).
Compared to the original hyper-polygraph, 
the value of $(\totalsize{\wwcons_p} + \totalsize{\wrcons_p})$ -- 
which equals the number of boolean variables --
is usually effectively reduced due to pruning.

\inlsec{Solving} 
Analyzing the complexity of SMT solvers is inherently challenging~\cite{Flexible:book2022,Tractability:book2014,ProofComplexity:CAV2018}. 
In this work, 
we rely on a somewhat simplistic model~\cite{SMT:JACM2006}: 
\[ \SMTcost \approx \SATcost + \sum_{i = 0}^{N_{\alpha}} \theorycost(\alpha_i). \]
In this model, 
the time complexity of an SMT solver (denoted by $\SMTcost$) 
is decomposed into two components:  
(1) the cost of the SAT solver (denoted by $\SATcost$), and 
(2) the cost of invoking the theory solver to check $i$-th assignment $\alpha_i$ 
(denoted by $\theorycost(\alpha_i)$)\footnote{
It is important to note that 
the costs of the SAT solver and the theory solver 
cannot be simply added together, 
as the theory solver may greatly influence the solving procedure of the SAT solver~\cite{HandbookMC:book2018}.
}.
The upper bound for $\SATcost$ is $2^{\cardinality{\cvars}}$ 
(i.e., $2^{\totalsize{\wwcons_p} + \totalsize{\wrcons_p}}$).
In practice, 
$\SATcost$ is heavily influenced by the number of conflicts 
encountered during solving~\cite{Empirical:book2013}. 

Given an assignment $\alpha_i$, 
the theory solver first derives $\RW$ edges 
based on the assigned variables, 
and then applies the PK algorithm to detect cycles for each edge.
We denote the \emph{affected region} of edge $(T, S)$ in $\ug$ by $\delta_{T, S}$, 
which is defined as 
$\delta_{T, S} = \set{S' \mid \clevel{S} < \clevel{S'} \land S \leadsto_{\ug} S'} \cup 
\set{T' \mid \clevel{T'} < \clevel{T} \land T' \leadsto_{\ug} T}$. 
We also use $\llangle \delta_{T, S} \rrangle$ to represent the number of search steps required.
The cost of inserting an edge $(T, S)$ and invoking the PK algorithm is 
$O(\cardinality{\delta_{T, S}}\log (\cardinality{\delta_{T, S}}) + \llangle \delta_{T, S} \rrangle)$~\cite{PKTopo:ACMJEA2006}.
Therefore, the cost of the theory solver for an assignment $\alpha_i$ is:
\[
\theorycost(\alpha_i) = 
\left\{\begin{matrix}
O(1)  &  \text{ if } \alpha_i \text{ is negative }  \\
\sum\limits_{\cwrvar{x}_{T, S} \in \pa} \cardinality{\delta_{S, T'}}\log(\cardinality{\delta_{S, T'}}) + \llangle \delta_{S, T'} \rrangle   & \text{ if } \alpha_i \triangleq \cwwvar_{T, T'}^x \\  
\sum\limits_{\cwwvar_{T, T'}^x \in \pa} \cardinality{\delta_{S, T'}}\log(\cardinality{\delta_{S, T'}}) + \llangle \delta_{S, T'} \rrangle   & \text{ if } \alpha_i \triangleq \cwrvar{x}_{T, S} \\  
\end{matrix}\right.
\]
The upper bound for invoking the theory solver once is 
$O(\cardinality{\V}\cdot (\cardinality{\V} + \cardinality{\E}))$. 
However, We contend again that this upper bound is rarely reached in practice.
This is primarily because  
approximately half of the assignments are negative 
(i.e., assigned $\false$), 
and most assignments satisfy the pseudo-topological order conditions, 
meaning that graph traversals are not required. 
Consequently, 
when consider the overall complexity, 
the amortized cost of invoking the theory solver does not pose a practical concern.

The above analysis also offers a new perspective to understand 
why our optimizations are effective.
By encoding 2-width cycles, 
\brown{certain} conflicts are pre-processed, 
and thereby avoided during solving.
This reduction not only decreases the $\SATcost$ 
but also lowers the number of assignments (denoted by $N_{\alpha}$), 
and it is the latter effect that consequently reduces the number of calls to the theory solver.
Although precisely analyzing the impact of the polarity picking is 
beyond our capability~\cite{Complexity:TOCL2006}, 
we nevertheless observe that this strategy helps reduce the number of conflicts 
(see Section~\ref{subsubsec:impact-polarity}), 
playing a role analogous to that of encoding 2-width cycles.
