# Supplementary material for: Fast Verification of Strong Database Isolation (Extended Version)
Source: arXiv:2511.14067 source file (2025-11-18)
Supplement: Supplementary file 2 [file app-gpu-eval-wo-pro6000.tex]

% app-gpu-eval-wo-pro6000.tex

\section{\textcolor{ForestGreen}{Comparison with Cobra Equipped with a More Powerful GPU}}
\label{section:appendix-gpu}

\reviewleft{Meta}{4}{ForestGreen}{
Cobra leverages GPUs to accelerate reachability computation during pruning.
To further assess whether more powerful GPUs can improve the checking process, 
we compare \ourtool with Cobra run on servers equipped with different GPUs. 
Due to resource limitations, 
a unified CPU configuration is not available, 
and thus the experiments are conducted on two distinct servers, 
each identified by its GPU model:
\begin{enumerate}
  \item \textbf{H800}. Intel Xeon Platinum 8454P CPU, NVIDIA H800 GPU, and 100GB of RAM.
  \item \textbf{V100}. Intel Xeon Platinum 8163 CPU, NVIDIA V100 GPU, and 32GB of RAM.
\end{enumerate}
}

\textcolor{ForestGreen}{
In general, 
the \textbf{H800} server has a higher computational capacity 
than \textbf{V100} for both CPUs and GPUs.
We run Cobra on them  
and run \ourtool on the \textbf{H800} server.
Figure~\ref{fig:gpu} shows the runtime comparison of Cobra and \ourtool.
}

% gpu.tex

\pgfplotsset{height=140pt, width=240pt}
\pgfplotsset{tick style={draw=none}}
\begin{figure}[h]
	\centering
	\resizebox{.5\linewidth}{!}{
%		\begin{minipage}{0.31\textwidth}
		\begin{scaletikzpicturetowidth}{\textwidth}
			\begin{tikzpicture}[scale=\tikzscale]
				\begin{axis}[
					font=\LARGE,
					xlabel={\#txns},
					xtick={1000,4000,6000,8000,10000,12000,14000,16000},
					xticklabels={1k,4k,6k,8k,10k,12k,14k,16k},
					xticklabel style={/pgf/number format/fixed},
					scaled x ticks=false,
					ylabel={Time (s)},
					ymax=51,
					ytick={0,10,20,50},
					cycle multiindex* list={
									color       \nextlist
									mark list*  \nextlist
							},
						legend pos=north west,
            legend style={xshift=1pt, yshift=1pt,draw=none},
					height=170pt,
					]
					\addplot[color=blue,mark=o,mark size=3pt] table [x=param, y=ours, col sep=comma] {figs/eval/gpu/end-to-end.csv};
					% \addplot[color=brown,mark=square,mark size=3pt] table [x=param, y=cobra(w/pro6000), col sep=comma] {figs/eval/gpu/end-to-end.csv};
					\addplot[color=brown,mark=square,mark size=3pt] table [x=param, y=cobra(w/v100), col sep=comma] {figs/eval/gpu/end-to-end.csv};
					\addplot[color=magenta,mark=Mercedes star,mark size=3pt] table [x=param, y=cobra(w/h800), col sep=comma] {figs/eval/gpu/end-to-end.csv};
					\legend{\ourtool, \cobra(\textbf{V100}), \cobra(\textbf{H800})}
				\end{axis}
			\end{tikzpicture}
		\end{scaletikzpicturetowidth}
%	\end{minipage}
	
%	\begin{minipage}{0.31\textwidth}
%		\begin{scaletikzpicturetowidth}{\textwidth}
%			\begin{tikzpicture}[scale=\tikzscale]
%				\begin{axis}[
%					font=\LARGE,
%					title={(b) Avg. Time of Computing Reachability},
%					xlabel={\#txns},
%					xtick={1000,4000,6000,8000,10000,12000,14000,16000},
%					xticklabels={1k,4k,6k,8k,10k,12k,14k,16k},
%					xticklabel style={/pgf/number format/fixed},
%					scaled x ticks=false,
%					ylabel={Time (s)},
%					ymax=5,
%					% ytick={0,10,20,50,100},
%					cycle multiindex* list={
%									color       \nextlist
%									mark list*  \nextlist
%							},
%						legend pos=north west,
%            legend style={xshift=1pt, yshift=1pt,draw=none},
%					height=170pt,
%					]
%					\addplot[color=blue,mark=o,mark size=3pt] table [x=param, y=ours, col sep=comma] {figs/eval/gpu/reachability.csv};
%					% \addplot[color=brown,mark=square,mark size=3pt] table [x=param, y=cobra(w/pro6000), col sep=comma] {figs/eval/gpu/reachability.csv};
%					\addplot[color=green!50!black,mark=asterisk,mark size=3pt] table [x=param, y=cobra(w/h800), col sep=comma] {figs/eval/gpu/reachability.csv};
%					\addplot[color=violet,mark=triangle,mark size=3pt] table [x=param, y=cobra(w/v100), col sep=comma] {figs/eval/gpu/reachability.csv};
%					% \legend{\ourtool, \cobra(\textbf{PRO6000}), \cobra(\textbf{H800}), \cobra(\textbf{V100})}
%					\legend{\ourtool, \cobra(\textbf{H800}), \cobra(\textbf{V100})}
%				\end{axis}
%			\end{tikzpicture}
%		\end{scaletikzpicturetowidth}
%	\end{minipage}

	}
	\captionsetup{skip=2pt}
	\caption{Verification time: \ourtool vs Cobra with different GPU capabilities.} 
	% on the BlindW-RW dataset of 10k keys.}
	
	\label{fig:gpu}
	\vspace{-2ex}
\end{figure}

% \textcolor{ForestGreen}{
% Figure~\ref{fig:gpu}(a) shows the average time of 
% a single reachability computation during pruning.
% Because the number of passes varies, 
% we measure the average cost of one reachability computation.
% The results show that computation time of Cobra  
% does not differ significantly across settings, 
% but in all cases it is higher than that of \ourtool.
% This observation is particularly intriguing, 
% given that these GPUs typically 
% exhibit notable performance differences in deep learning tasks.
% To investigate it, 
% we monitor the peak real-time power consumption of the GPUs, 
% which turns out to be far below their theoretical maximum.
% This suggests that employing a more powerful GPU provides limited benefit, 
% as the peak demand of the acceleration algorithm has already been saturated.
% Under such conditions, 
% the performance of reachability computation may be 
% constrained by other system components, 
% such as CPU capacity or memory latency.
% This may also explain why the H800 GPU exhibits lower performance than the V100.
% \brown{We acknowledge that modern GPUs could be better exploited 
% through careful algorithmic design and optimized implementations.
% Nevertheless, for current and commonly encountered workloads in history-checking, 
% it is sufficient to employ our reachability algorithm, 
% which achieves comparatively better performance without relying on high-end GPUs.}
% }

\textcolor{ForestGreen}{
Figure~\ref{fig:gpu} shows the comparison of end-to-end checking time.
\ourtool outperforms Cobra even when Cobra uses more powerful GPUs.
This improvement arises because GPUs are not the bottleneck of checking time 
and the main overhead is on solving rather than pruning.
The dedicated SMT solver integrated into \ourtool is specifically optimized 
based on the characteristics of workloads, 
and thus performs better than MonoSAT directly employed by Cobra.
% Another noteworthy observation is that 
% Cobra appeared to run somewhat faster on \textbf{PRO6000} than on the other two servers.
% This improvement is likely attributable to the improved CPU performance, 
% and it may also provide supportive evidence for our earlier hypothesis 
% that GPUs are not the bottleneck in this task.
}

% \textcolor{ForestGreen}{
% In summary, solving rather than pruning constitutes the dominant overhead in checking. 
% with pruning accelerated by GPUs while solving remains independent of them.
% Our approach remains efficient primarily 
% because of the dedicated solver.
% \brown{
% Since reachability computation is a fundamental component, 
% advances in GPU capabilities or breakthroughs in underlying algorithms 
% may eventually render our current reachability method insufficient.
% At that stage, however, our framework can readily employ such advances 
% to further improve performance. \zhiheng{may not need}}
% }
