# Supplementary material for: Fast Verification of Strong Database Isolation (Extended Version)
Source: arXiv:2511.14067 source file (2025-11-18)
Supplement: Supplementary file 3 [file app-list-proof.tex]

\section{Proof Sketch of General List-append}

\blue{[move it into preliminaries]}
For a total order $R$, 
if $a \rel{R} b$ and there is no such $c$ that $a \rel{R} c \rel{R} b$, 
we call $(a, b)$ is an \emph{immediate} element of $R$,
denoted as $a \relimm{R} b$.

\subsection{Definition}

We modify Theorem~\ref{def:si-axiomatic} to formalize the \ser of list-append histories.
%%%%%%%%%%%%%%%%%%%%
\begin{definition}[\ser~\cite{Framework:CONCUR2015}]
  \label{def:si-axiomatic-list}
	A list-append history $\h = (T, \SO)$ satisfies \ser{} if and only if
  there exists an abstract execution $\ae = (T, \SO, \vis, \ar)$
  such that the $\sessionaxiom$, $\intextaxiom$,
	and $\totalvis$ axioms hold.
\end{definition}

Since a read operation of transaction $T$ 
may read from both internal and external of $T$, 
we merge the \intaxiom{} and \extaxiom{} axioms into the \intextaxiom{} axiom, 
leaving \sessionaxiom{} and \totalvis{} axioms unchanged 
(they are irrelevant to the semantics of lists).
Let \emph{global arbitration} (denoted as $\gar$) 
extend $\ar$ to the operation level with $\po$ of transactions: 
$\gar \triangleq (\bigcup\limits_{T \in \T} \po_T \cup \bigcup\limits_{T \rel{\ar} S} O_T \times O_S)^{+}$ 
is still a total order over $\allops$.
Let \emph{global visibility} (denoted as $\gvis$) 
extend $\vis$: 
$\gvis \triangleq \bset{(o_1, o_2) \mid o_1 \in T \land o_2 \in S \land (T, S) \in \vis} \cup \bigcup\limits_{T \in \T} \po_T$.
The \intextaxiom{} axiom requires that 
for each read operation $r \triangleq \readevent(x, [v_1, v_2, \cdots, v_n])$, 
there exists exactly $n + 1$ append operations in $\gvis^{-1}(r) \cap \set{\appendevent(x, \_)}$.
Let $w_0, w_1, \cdots, w_n$ denote these operations in the order of $\gar$ 
(i.e., $w_0 \rel{\gar} w_1 \rel{\gar} w_2 \rel{\gar} \cdots \rel{\gar} w_{n}$),
they must satisfy $w_0 \triangleq \appendevent(x, \emptyset)$ and
$\forall 1 \leq i \leq n.\; w_i \triangleq \appendevent(x, v_i)$. 
%%%%%%%%%%%%%%%%%%%%

\subsection{Proof of Theorem~\ref{thm:ser-uupg}}

\begin{proof}
  We prove Theorem~\ref{thm:ser-uupg} in two directions.

  (``$\Leftarrow$'') 
  Suppose there exists an compatible graph $\G'$ of the unfolded universal polygraph of a history $\H$
  such that $\G'$ is acyclic and $(\G' - \unfoldedreadops) / \txnequivalence$ is acyclic.
  We then construct $\vis$ and $\ar$ such that 
  (1) they are well-defined, i.e., $\vis$ is acyclic, $\ar$ is total and $\vis \subseteq \ar$; and  
  (2) they satisfy \sessionaxiom{}, \intextaxiom{} and \totalvis{} axioms.
  Nodes of $(\G' - \unfoldedreadops) / \txnequivalence$ correspond to transactions of $\H$.
  Let $\ar$ be an topological order of $(\G' - \unfoldedreadops) / \txnequivalence$ and 
  set $\vis = \ar$, the following properties are hold straghtforwardly:
  \begin{enumerate}
    \item (well-defined) $\vis$ is acyclic, $\ar$ is total, and $\vis \subseteq \ar$;
    \item (\sessionaxiom{}) $\SO \subseteq \ar$, 
      where $\SO$ is a subset of edges from $(\G' - \unfoldedreadops) / \txnequivalence$;
    \item (\totalvis{}) $\vis = \ar$ and $\ar$ is total;
  \end{enumerate} 

  Next, consider the \intextaxiom{} axiom.
  Let $r \triangleq \readevent(x, [v_1, v_2, \cdots, v_n])$ be an arbitary read operation.
  Its unfolded reads in $\G'$ are denoted by 
  $r'_0 \rel{\app(x)} r'_1 \rel{\app(x)} \cdots \rel{\app(x)} r'_{n - 1} \rel{\app(x)} r$. 
  Let $w_0, w_1, \cdots, w_n$ be the corresponding write operations in $\WR(x)^{-1}$ 
  for $r'_0, r'_1, \cdots, r'_{n - 1}$ and $r$, respectively.
  We know that:
  $$w_0 \relimm{\WW(x)} w_1 \relimm{\WW(x)} w_2 \relimm{\WW(x)} \cdots \relimm{\WW(x)} w_n \rel{\WR(x)} r,$$ 
  so that $\gvis^{-1}(r) \cap \set{\appendevent(x, \_)}$ contains at least $n + 1$ elements:  
  $w_0, w_1, \cdots, w_n$.
  We now show that there is no other write operation $w'$ in $\gvis^{-1}(r) \cap \set{\appendevent(x, \_)}$. 
  Since $w_0$ is the initial write and 
  there are no intermediate write operation between any of $w_i$ and $w_{i + 1}$,
  if such a $w'$ exists, it must satisfies $w_n \rel{\WW(x)} w'$.
  We apply the $\RW$ derivation rule:
  $$w_n \rel{\WW(x)} w' \land w_n \rel{\WR(x)} r \implies r \rel{\RW(x)} w',$$ 
  which contradicts the visibility of $w'$ to $r$.
  Finally, we show that $w_0 = \appendevent(x, \emptyset)$ and 
  $\forall 1 \leq i \leq n.\; w_i = \appendevent(x, v_i)$.
  This is guaranteed by the definition of $\WR$ edges.
  Thus all conditions of \ser hold, and we conclude $\H \models \ser$.

  (``$\Rightarrow$'') 
  Suppose there exist $\vis$ and $\ar$ for a history $\H$ such that 
  $\vis$ is acyclic, $\ar$ is total, and $\vis \subseteq \ar$; and 
  they satisfy \sessionaxiom{}, \intextaxiom{} and \totalvis{} axioms.

  An important conclusion here is that $\vis = \ar$, 
  this is ensured by the \totalvis{} axiom.
  Spefically,
  if $(T, S) \in \ar$ but $(T, S) \notin \vis$,
  then $(S, T) \in \vis$, 
  which constradicts $\vis \subseteq \ar$.
  
  Next, we construct a compatible graph of the unfolded universal polygraph of $\H$ 
  using $\vis$ and $\ar$ in two steps.
  In the first step, we exclude those unfolded read operations out of consideration: 
  \footnote{
    Note that through $\vis$ and $\ar$ are equal here, 
    we maintain the distinction, 
    aimming at providing this proof as an outline for \si. 
  }
  \begin{enumerate}
    \item $\po$ and $\SO$: Add the $\po$ and $\SO$ edges directly from $\H$;
    \item $\WW$: For each pair of write operations $w$ and $w'$ that write the same key $x$, 
      if $w \rel{\gar} w'$ then add $w \rel{\WW(x)} w'$.
    \item $\WR$: For each read $r \triangleq \readevent(x, \_)$, 
      let $w = \max_{\gar}(\gvis^{-1}(r) \cap \set{\appendevent(x, \_)})$ 
      ($w$'s existence is guaranteed by the \intextaxiom{} axiom). 
      Add $w \rel{\WR(x)} r$.
    \item $\RW$: After steps (1), (2) and (3), 
      add derived $\RW$ edges based on the $\WW$ and $\WR$ edges.
  \end{enumerate}

  We denote the resulting graph as $\G'_1$.
  $\G'_1$ satisfies the definitions of $\WW$, $\WR$ and $\RW$.
  We now show that \textbf{$\G'_1$ is acyclic}.
  To show the acyclicity of $\G'_1$, 
  observe that $\po$, $\SO$, $\WW$ and $\WR$ edges do not contradict $\gar$ by definition, 
  and the same holds for $\RW$.
  If $r \rel{\RW(x)} w'$ forms a cycle, 
  it must be derived from some $w$ and $r$ such that 
  $w \rel{\WR(x)} r$ and $w \rel{\WW(x)} w'$.
  Since $\gar$ is total, we know $w' \rel{\gar} r$, 
  which implies $w' \rel{\gvis} r$ and $w \rel{\gar} w'$.
  This contradicts the maximality of $w$ in $(\gvis^{-1}(r) \cap \set{\appendevent(x, \_)})$.  
  Thus $\G'_1$ is acyclic, and so is $\G'_1 / \txnequivalence$, 
  since every edge in $\G'_1$ connecting two transactions does not contradict $\ar$.

  Now we add $\unfoldedreadops$ to $\G'_1$ to construct the complete compatible graph: 
  \begin{enumerate}
    \item $\app$: Add the $\app$ edges by definition;
    \item $\WR$: For each read operation $r \triangleq \readevent(x, \_)$, 
    consider the elements of $\gvis^{-1}(r) \cap \set{\appendevent(x, \_)}$.
    Add the edges $w_0 \rel{\WR(x)} r'_0$, $w_1 \rel{\WR(x)} r'_1$, $\cdots$, $w_{n - 1} \rel{\WR(x)} r'_{n - 1}$.
    \item $\RW$: After step (2), add new derived $\RW$ edges based on existing $\WW$.
  \end{enumerate}
  We denote the graph after this second construction as $\G'_2$.
  $\G'_2$ satisfies the definitions of $\app$ and newly added $\WR$ and $\RW$ edges. 
  
  Next, we show that: 
  \begin{enumerate}
    \item $\G'_2$ satisfies the derivation rule of $\app$.
    \item $\G'_2$ is still acyclic.
  \end{enumerate} 

  For (1), consider $w, w', r, r'$ such that 
  $w \rel{\WR(x)} r \land w' \rel{WR(x)} r' \land r \rel{\app(x)} r'$.
  From \intextaxiom{}, we know that $w \rel{\WW(x)} w'$.
  If there exists $w''$ such that $w \rel{\WW(x)} w'' \rel{\WW(x)} w'$, 
  then $w''$ must be in $(\gvis^{-1}(r) \cap \set{\appendevent(x, \_)})$, 
  which contradicts \intextaxiom{} either.

  For (2), we first show that 
  if an unfolded read operation $r'_i$ is part of a cycle in $\G'_2$,
  then there also exists a cycle in $\G'_2$ that does not include $r'_i$.
  Consider the unfolded read operations of a read operation $r$: 
  $$r'_0 \rel{\app(x)} r'_1 \rel{\app(x)} \cdots \rel{\app(x)} r'_{n - 1} \rel{\app(x)} r,$$
  and suppose $r'_i$ is in a cycle.
  As shown in Figure~\ref{fig:list-proof}, edges near $r'_i$ are as follows: 
  \begin{itemize}
    \item $r'_i$ has at most two outer edges: 
      $r'_i \rel{\app(x)} r'_{i + 1}$ and $r'_i \rel{\rw(x)} w_{i + 1}$,
    \item $r'_i$ has at most two inner edges: 
    $r'_{i - 1} \rel{\app(x)} r'_i$ and $w_i \rel{\app(x)} r'_i$.
  \end{itemize}
  If the cycle contains $r'_{i - 1}$ and the $\app$ edge $r'_{i - 1} \rel{\app(x)} r'_i$, 
  we can trace the cycle backward through $\app(x)$ edges 
  until we reach some $r'_j$ where $r'_{j - 1}$ is not in the cycle.
  In this case, $w_j$ must be part of the cycle.

  Now consider the outer edges of $r'_i$.
  If $r'_i \rel{\app(x)} r'_{i + 1}$ is in the cycle, 
  then the path 
  $$w_j \rel{\ww(x)} \cdots \rel{\ww(x)} w_i \rel{\ww(x)} w_{i + 1} \rel{\wr(x)} r'_{i + 1} \rel{} \cdots \rel{} w_j$$ 
  forms a cycle; 
  Similarly, if $r'_i \rel{\rw(x)} w_{i + 1}$ is in the cycle, 
  then $$w_j \rel{\ww(x)} \cdots \rel{\ww(x)} w_i \rel{\ww(x)} w_{i + 1} \rel{} \cdots \rel{} w_j$$
  also forms a cycle.
  Thus if a cycle includes an unfolded read operation,
  then there must exists a cycle that do not contain any read operation.
  These cycles are also present in $\G'_1$ too.
  Given that $\G'_1$ is acyclic, $\G'_2$ is acyclic too.
  Therefore we construct a valid compatible graph of $\H$.
\end{proof}

\begin{figure}[t]
  \centering
  \includegraphics[width=\columnwidth]{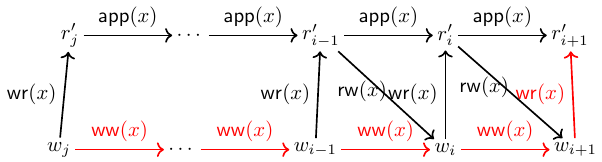}
  \caption{Construction of a cycle in $\G'_1$}
  \label{fig:list-proof}
\end{figure}
