# Supplementary material for: Fast Verification of Strong Database Isolation (Extended Version)
Source: arXiv:2511.14067 source file (2025-11-18)
Supplement: Supplementary file 4 [file other-opts.tex]

% \section{Misc}

% \subsection{Other Optimizations} \label{subsec:other-opts}

% exactly-one-encoding.tex

\begin{figure}[t]
  \centering
  \begin{subfigure}[b]{0.20\textwidth}
    \centering
    \includegraphics[width=0.8\textwidth]{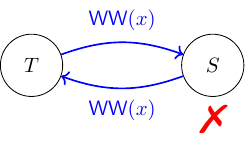}
       		        		\captionsetup{skip=2pt}
    \caption{For $\WW$ constraints}
    \label{fig:exactly-one-encoding-ww}
  \end{subfigure}
\hspace{4ex}
  \begin{subfigure}[b]{0.2\textwidth}
    \centering
    \includegraphics[width=0.8\textwidth]{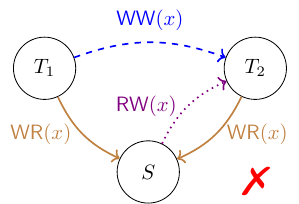}
       		        		\captionsetup{skip=2pt}
    \caption{For $\WR$ constraints}
    \label{fig:exactly-one-encoding-wr}
  \end{subfigure}
     		        		\captionsetup{skip=4pt}
  \caption{Illustration of the ``at-most-one''
    parts of $\WW$ and $\WR$ constraints.}
  \label{fig:exactly-one-encoding}
\end{figure}
\begin{algorithm}
  \footnotesize
  \caption{Theory Propagate}
  \label{algo:theory-propagate}
  \begin{algorithmic}[1]
    \Function{TheoryPropagate }{$\pa$}
      \ForAll{$\cwrvar{x}_{T, S} \in \pa$ for some $x, T$ and $S$}
        \State{$\pa \gets \pa \cup 
                \set{\lnot \cwrvar{x}_{T', S} \mid 
                     \exists \ccons \in \wrcons.\;T' \rel{\WR(x)} S \in \ccons 
                \land T \neq T' \land \cwrvar{x}_{T', S} \text{ is unassigned}}$}
      \EndFor
      \State{\Return $\pa$}
    \EndFunction
  \end{algorithmic}
\end{algorithm}

\inlsec{Encoding Exactly-One Constraints} %\label{sss:theory-propagate}
Both $\WW$ and $\WR$ constraints take the form of ``exactly-one'' constraints, typically written as a pseudo-boolean formula $x_1 + x_2 + \cdots + x_n = 1$, where $x_i$  is either 0 ($\false$) or 1 ($\true$)~\cite{SAT-Handbook}. While encoding this into CNF requires $O(n^2)$ clauses, we observe that the “at-most-one” part (i.e., $x_1 + \cdots + x_n \leq 1$) can be safely omitted due to the acyclicity requirement.

Take $\WR$ constraints in Figure~\ref{fig:exactly-one-encoding-wr} for example.
Suppose that $T_{1} \rel{\WW(x)} T_{2}$, 
both $T_{1} \rel{\WR(x)} S$ and $T_{2} \rel{\WR(x)} S$ hold.
Then we have $S \rel{\RW(x)} T_{2}$,
forming a cycle $S \rel{\RW(x)} T_{2} \rel{\WR(x)} S $.

Dropping the ``at-most-one'' part disables automatic unit propagation: once a variable $x_i$ is assigned $\true$, the SAT solver can no longer infer that all other variables must be $\false$. 
To compensate, we reimplement this as a theory  propagation strategy in \ourtool's backend;
see the Appendix for details.
\nobi{this section is hard to follow}
