# Supplementary material for: Fast Verification of Strong Database Isolation (Extended Version)
Source: arXiv:2511.14067 source file (2025-11-18)
Supplement: Supplementary file 5 [file si.tex]

% si.tex

\begin{definition}[Snapshot Isolation
	(Axiomatic)~\cite{Framework:CONCUR2015, AnalysingSI:JACM2018}]
  \label{def:si-axiomatic}
	A history $\h = (T, \SO)$ satisfies SI if and only if
  there exists an abstract execution $\ae = (T, \SO, \vis, \ar)$
  such that the $\sessionaxiom$, $\intaxiom$, $\extaxiom$,
	$\prefixaxiom$, and $\noconflictaxiom$ axioms (explained below) hold.
\end{definition}

\footnote{
That is, we consider the \emph{strong session} variant
of \si{}~\cite{LazyReplSI:VLDB2006, AnalysingSI:JACM2018}
commonly used in practice.}

The \prefixaxiom{} axiom (i.e., $\ar \comp \vis \subseteq \vis$) ensures that
if the snapshot taken by a transaction $T$ includes a transaction $S$,
than this snapshot also include all transactions that committed before $S$
in terms of $\ar$.
The \noconflictaxiom{} axiom
prevents concurrent transactions from writing on the same key.
That is, for any conflicting transactions $S$ and $T$,
one of $S \rel{\vis} T$ and $T \rel{\vis} S$ must hold.

\begin{example}
  \label{ex:si}

  Figure~\ref{fig:si-op-axiomatic} shows that the history
  is also valid under the axiomatic semantic of SI.
  It constructs a possible abstract execution
  by establishing the visibility and arbitration relations
  as shown in the figure.
  For example, $T_{0}$ is visible to $T_{2}$ but $T_{1}$ is not.
  Both $T_{0}$ and $T_{1}$ are visible to $T_{3}$.
  Since $T_{1}$ is after $T_{0}$ in terms of $\ar$,
  $T_{3}$ reads the value 2 of $y$ written by $T_{1}$.
\end{example}

In contrast to \ser, \si permits specific cycle patterns while prohibiting other general cycles.

\begin{theorem}[Dependency Graph-based Characterization of \si{}
    (Theorem 4.1 of~\cite{AnalysingSI:JACM2018})] \label{thm:depgraph-si}
  For a history \emph{$\H = (\T, \SO)$},
  \emph{\begin{align*}
    \H \models \si & \iff \H \models \intaxiom \;\land \\
      &\exists \WR, \WW, \RW.\; \G = (\H, \WR, \WW, \RW) \;\land \\
      &\quad (((\SO_{\G} \cup \WR_{\G} \cup \WW_{\G}) \comp \RW_{\G}?) \text{\it\; is acyclic}).
  \end{align*}}
\end{theorem}
