# Supplementary material for: Fast Verification of Strong Database Isolation (Extended Version)
Source: arXiv:2511.14067 source file (2025-11-18)
Supplement: Supplementary file 7 [file other-opt.tex]

\section{Encoding Exactly-One Constraints} 
\label{section:appendix-1-encoding}

% exactly-one-encoding.tex

\begin{figure}[t]
  \centering
  \begin{subfigure}[b]{0.20\textwidth}
    \centering
    \includegraphics[width=0.8\textwidth]{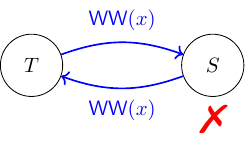}
       		        		\captionsetup{skip=2pt}
    \caption{For $\WW$ constraints}
    \label{fig:exactly-one-encoding-ww}
  \end{subfigure}
\hspace{4ex}
  \begin{subfigure}[b]{0.2\textwidth}
    \centering
    \includegraphics[width=0.8\textwidth]{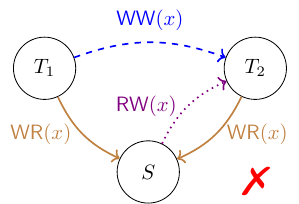}
       		        		\captionsetup{skip=2pt}
    \caption{For $\WR$ constraints}
    \label{fig:exactly-one-encoding-wr}
  \end{subfigure}
     		        		\captionsetup{skip=4pt}
  \caption{Illustration of the ``at-most-one''
    parts of $\WW$ and $\WR$ constraints.}
  \label{fig:exactly-one-encoding}
\end{figure}
