# Supplementary material for: Fast Verification of Strong Database Isolation (Extended Version)
Source: arXiv:2511.14067 source file (2025-11-18)
Supplement: Supplementary file 8 [file si-upg.tex]

% si-upg.tex

\subsection{Characterizing \si}

Based on the \bfit{induced SI graph} of PolySI\cite{PolySI:VLDB2023},
we can simply extend our characterization of general \rwregisters{} histories to \si.

%%%%%%%%%%%%%%%%%%%%
\begin{definition} \label{def:si-acyclic}
  Let $G = (V, E, C)$ be a universal polygraph of a history $\H$.
  If there exists at least one compatible graph
  and its induced SI graph is acyclic when edge types and keys are ignored,
  then $G$ is \bfit{\si-acyclic}.
\end{definition}
%%%%%%%%%%%%%%%%%%%%

%%%%%%%%%%%%%%%%%%%%
\begin{theorem}[Universal Polygraph-based Characterization of \si{}] \label{thm:universal-polygraph-si}
  A history $\H$ satisfies \emph{\si{}} if and only if
  \emph{$\H \models \intaxiom$} and the universal polygraph of $\H$ is \si-acyclic.
  \zhiheng{remove \intaxiom{} here and add it into implementation}
\end{theorem}
%%%%%%%%%%%%%%%%%%%%

The difference between the definition of generalized-polygraph-based and universal-polygraph-based induced SI graphs
can be found in \cite[Appendix XX]{tech-rpt}.
