# Supplementary material for: Fast Verification of Strong Database Isolation (Extended Version)
Source: arXiv:2511.14067 source file (2025-11-18)
Supplement: Supplementary file 9 [file app-list-proof-old.tex]

\section{Proof Sketch of General List-append}

\subsection{The Characterization Theorem}

\inlsec{Notations}
We use $l$ to denote lists, where $l = [v_1, v_2, \cdots, v_n]$, 
$n$ is the length of $l$ (also denoted as $|l|$). 
$l_{-1}$ is used to denote the last element $l_n$.
If $l_1 = [v_1, v_2, \cdots, v_n]$ and $l_2 = [v'_1, v'_2, \cdots, v'_m]$, 
we call $l_1 = l_2$ iff $n = m$ and $v_1 = v'_1, v_2 = v'_2, \cdots, v_n = v'_m$.
We use $l_{:i}$ to denote the prefix of $l$ with length $i$, that is $l_{:i} = [v_1, v_2, \cdots, v_i]$.
In a list-append history $\H = (\T, \SO)$, we use $\readlists$ to denote the set of all lists that is read in a read event.
Formally, $\readlists = \set{l | \exists \keyxvar \in \Key, T \in \T.\; T \vdash \readevent(\keyxvar, l)}$.

\inlsec{Theorem}
\begin{definition}
  A dependency graph $\G = (\H, \WR, \WW, \RW)$ \bfit{agrees with} the corresponding $\H$, if 
  $\forall \keyxvar \in \Key.\; \forall S \vdash \readevent(\keyxvar, l).$

  \blue{[TODO: $T_1 \rel{\WW(x)} T_2 \rel{\WW(x)} \cdots T_n \rel{\WR(x)} S. S \vdash \readevent(x, l),
T_1 \vdash \writeevent(x, v_1), T_2 \vdash \writeevent(x, v_2), \cdots, T_n \vdash \writeevent(x, v_n). l = [v_1, v_2, \cdots, v_n]$]}
\end{definition}

\begin{theorem}[Dependency Graph-based Characterization of \ser{} for list-append histories] \label{thm:depgraph-ser-list}
  For a list-append history \emph{$\H = (\T, \SO)$},
  \emph{\begin{align*}
    \H \models \ser & \iff \H \models \intaxiom \;\land \\
      &\exists \WR, \WW, \RW.\; \G = (\H, \WR, \WW, \RW) \;\land \\
      &\quad ((\SO_{\G} \cup \WR_{\G} \cup \WW_{\G} \cup \RW_{\G}) \text{\it\; is acyclic}) \;\land \\
      &\G \text{\it\; agrees with } \H.
  \end{align*}}
\end{theorem}

\subsection{Proof Sketch}

\inlsec{Proof Target}
(If $\H \not\models \intaxiom \lor \H \not\models \listprefixaxiom$, then $\H \not\models \ser$),
$\H \models \ser \iff $ exists a directed labeled graph with relating keys 
that is compatible with the universal polygraph of $\Hplus$.

\begin{lemma} \label{lem:hplus-ser}
  (If $\H \models \intaxiom \land \H \models \listprefixaxiom$, )  
  $\Hplus \models \ser \iff \H \models \ser$.
\end{lemma}

\begin{proof}
  \begin{enumerate}
    \item \bfit{$\Hplus \models \ser \implies \H \models \ser$}.
    $\Hplus \models \ser \implies \exists \Gplus.$ that satisfies Theorem~\ref{thm:depgraph-ser-list}.
    $\G$ can be constructed from deleting those $(T, S)$ that satisfies $T \in \observers(\H) \lor S \in \observers(\H)$.
    Then $\H \models \ser$. 

    \item \bfit{$\H \models \ser \implies \Hplus \models \ser$}.
    $\H \models \ser \implies \exists \G.$ that satisfies Theorem~\ref{thm:depgraph-ser-list}.
    $\Gplus$ can be constructed from $G$, 
    for all $T_1 \rel{\WW(x)} T_2 \rel{\WW(x)} \cdots T_n \rel{\WR(x)} S. S \vdash \readevent(x, l)$.
    Suppose that $l = [v_1, v_2, \cdots, v_n]$ and $O_1, O_2, \ldots, O_n \in \observers(\H). \;O_1 \vdash \readevent(x, l_{:1}), O_2 \vdash \readevent(x, l_{:2}), \cdots, O_n \vdash \readevent(x, l_{:n})$.
    Let $T_1 \rel{\WR(x)} O_1, T_2 \rel{\WR(x)} O_2, \cdots, T_n \rel{\WR(x)} O_n$.
    Spefically, if $O_{n + 1}$ exists, i.e. $S \vdash \writeevent(x, v_{n + 1})$, 
    $S \rel{\WR(x)} O_{n + 1}$ to $\Gplus$ is then added to $\Gplus$.
    Considering that all observers are the end of paths (i.e. no outer edges), 
    this construction would not introduce cycles and keep the agreement with $\H$.
    \blue{[The uniqueness of $\WR$ edges are ensured by the definition of $T_1 \rel{} T_2 \cdots \rel{} T_n$]}.
  \end{enumerate}
\end{proof}

Lemma~\ref{lem:hplus-ser} moves the proof target to 
$\Hplus \models \ser \iff$ exists a directed labeled graph (with relating keys) 
that is compatible with the universal polygraph of $\Hplus$.

\begin{proof}
  \begin{itemize}
    \item \bfit{$\Leftarrow$}:  
    Let $\G$ be the compatible graph of the UP of $\Hplus$, 
    construct $\G'$ by deleting $\LO$ edges of $\G$.
    $\G$ is acyclic and $\land \E' \subseteq \E$ implies that $G'$ is also acyclic.
    For each read value $l$, $E'$ contains observers of all prefixes of $l$.
    The agreement can be inductively constructed.
    The first step is to prove the agreement of all observers.
    Suppose that for $T_1 \rel{\WW(x)} T_2 \rel{\WW(x)} \cdots T_n \rel{\WR(x)} O_n$,
    $[v_1, v_2, \cdots, v_n] = l_{:n}$, 
    for $O_{n + 1} \vdash \readevent(x, l_{:n + 1})$, 
    adding $T_{n + 1} \rel{\WR(x)} O_{n + 1}$ to the end of sequence $T_i$ 
    (the $\LOtoWW$ property ensures $T_{n + 1}$ happens between $T_n$ and $O_{n + 1}$)
    meets the list equation condition.
    For those non-observer reads, the $\WRValue$ property ensures that the last write transaction 
    is the same as the corresponding observer.
    To summarize, $\G'$ is a valid dependency graph that satisfies theorem~\ref{thm:depgraph-ser-list}.

    \item \bfit{$\Rightarrow$}:
    $\Hplus \models \ser \implies$ there exists an acyclic dependency graph $\G$ of $\Hplus$.
    We first show that $\G$ satisfies the $\WRValue$ property.
    If $S$ and $S'$ reads the same value $l$ on a key $x$, we consider their previous write sequences
    $T_1  \rel{\WW(x)} T_2 \rel{\WW(x)}  \cdots T_n \rel{\WR(x)} S$ and 
    $T'_1 \rel{\WW(x)} T'_2 \rel{\WW(x)} \cdots T'_{n'} \rel{\WR(x)} S'$.
    Since $S$ and $S'$ reads the same value $l$, $n$ must be equal to $n'$ (i.e. $|l|$).
    If $\exists T_k \neq T_k'.\;$, then either $T_k \rel{\WW(x)} T_k'$ or $T_k' \rel{\WW(x)} T_k$, 
    which contradicts the maximality of write sequences.
    Then we construct $\G'$ from $\G$ by adding $\LO$ edges.
    If $T \vdash \readevent(x, l_1), S \vdash \readevent(x, l_2), |l_1| < |l_2|$, 
    then we add $T \rel{\LO(x)} S$ into $\E'$.
    Note the the adding $\LO$ edges are a superset of $\LO$ edges in the universal polygraph.
    We will show that \circled{1} the adding $\LO$ edges do not form any cycle, 
    and \circled{2} $\G'$ satisfies the $\LOtoWW$ property.
    For \circled{2}, if there exists $T_1$, $T_2$, $S_1$ and $S_2$ such that 
    $T_1 \rel{\WR(x)} S_1$, $T_2 \rel{\WR(x)} S_2$, $S_1 \rel{\LO(x)} S_2$ but $T_2 \rel{\WW(x)} T_1$,
    then there exists $S_2 \rel{\RW(x)} T_1$, then we knows $S_2 \rel{\RW(x)} T_1 \rel{\WR(x)} S_1$.
    Note the edges are all in $\G$.
    Therefore the value read by $S_1$ (denoted as $l_1$) is longer than $S_2$ (denoted as $l_2$),
    contradicting to the construction rule of $\LO$ edges.
    For \circled{1}, we show that there is no cycle containing more than one $\LO$ edge.
    if there exists a cycle that contains $S_1 \rel{\LO(x)} S_2$, 
    since $\E'$ satisfies the $\LOtoWW$ property,
    we can substitute $S_1 \rel{\LO} S_2$ to $S_1 \rel{\RW(x)} T_2 \rel{\WR(x)} S_2$, 
    the cycle still exists in $\G$, which is contradicting.
    To summarize, $\G'$ is a valid compatible graph of the UP of $\Hplus$.
  \end{itemize}
\end{proof}
